# Supplementary material for: Optimal Gradient-based Algorithms for Non-concave Bandit Optimization
Source: arXiv:2107.04518 source file (2021-07-09)
Supplement: Supplementary file 1 [file proof_.tex]

\section{Proofs for $\cdots$}
